# Supplementary material for: Nanoparticle Taylor dispersion near charged surfaces with an open boundary
Source: arXiv:2206.07413 source file (2023-01-06)
Supplement: Supplementary file 1 [file supp.pdf]

# Supporting Information for: Nanoparticle Taylor dispersion near charged surfaces with an open boundary

Alexandre Vilquin,[1,2,*] Vincent Bertin,[1,3,4,*] Elie Raphaël,[1,2]
David S. Dean,[3,5] Thomas Salez,[3,†] and Joshua D. McGraw[1,2,‡]

[1] *Gulliver CNRS UMR 7083, PSL Research University, ESPCI Paris, 10 rue Vauquelin, 75005 Paris, France*
[2] *IPGG, 6 rue Jean-Calvin, 75005 Paris, France*
[3] *Univ. Bordeaux, CNRS, LOMA, UMR 5798, F-33405, Talence, France*
[4] *Physics of Fluids Group, Faculty of Science and Technology, and Mesa+ Institute, University of Twente, 7500AE Enschede, The Netherlands.*
[5] *Team MONC, INRIA Bordeaux Sud Ouest, CNRS UMR 5251, Bordeaux INP, Univ. Bordeaux, F-33400, Talence, France.*

(Dated: December 20, 2022)

* The authors contributed equally
† thomas.salez@cnrs.fr
‡ joshua.mcgraw@cnrs.fr

# I. VIDEO DESCRIPTIONS

- In Video S1 is shown a typical TIRFM image sequence with superimposed particle trajectories obtained with in-house particle-tracking software based on the `regionprops` function of MATLAB. The pressure imposed across the microfluidic system was 40 mbar with 150 mW laser illumination. The NaCl concentration was 5.4 mg/mL and the accumulated times since the initial frame are indicated.
- As shown in the snapshots of Fig. 1(b), Video S2 is a reconstruction of Video S1, with the origins of the displayed particles trajectories superimposed at a common point. A sample of 62 particles from each ensemble was used.

# II. MATERIALS AND METHODS

## A. Nanoparticles and flows in microchannels

In our objective-based, total internal reflection fluorescence microscope, we observed the motion of latex colloidal particles with radius $a = 55$ nm and density of $\rho = 1.1\ \mathrm{kg\,m^{-3}}$ (Fisher Scientific F8803). Such particles were advected by pressure driven flows with pressure drops between 20 and 70 mbar (Elveflow OB1). The microchannels were made with polydimethylsiloxane (Dow RTV) with a 20 $\mu$m height, 200 $\mu$m width and 8 cm length, and were sealed on a glass coverslip as a bottom surface. The particles' electrostatic interaction with this solid glass surface was tuned using the concentration of NaCl (Sigma) in ultrapure water (18.2 M$\Omega$ cm, MilliQ) independently measured by using a conductimeter (F30-Meter, Mettler-Toledo) and Kohlrauch's law for NaCl. Since these particles have similar density to water, we neglected the gravitational potential in the Gibbs-Boltzmann distribution, $c_{\mathrm{B}}$ in the main text. Indeed, the Boltzmann length is the typical vertical distance that a particle can be displaced under gravitational acceleration $g$ and random thermal motion. For water, this length is $L_{\mathrm{B}} = kT/\left(ga^3\Delta\rho\right) \approx 3$ cm, much larger that the typical size of the observation zone $\sim 1$ $\mu$m. Using dynamic light scattering (Malvern Zetasizer), we confirmed the particle size and measured the particle surface potential, $\psi_{\mathrm{p}} = -40 \pm 10$ mV. While this is lower than the values quoted in the main text, we verified that the resulting change on the predicted dispersion coefficients is never larger than 4 % percent on the overall decrease from the classical Taylor prediction.

## B. Total Internal Reflection Fluorescence Microscopy

Fluorescence of the nanoparticles was achieved using a continuous excitation laser (Coherent Sapphire, wavelength 488 nm) with the fluorescence intensity, $I$, related to the apparent particle altitude, $z_{\mathrm{app}}$, through $z_{\mathrm{app}} - a = \Pi \ln(I_0/I) \leq h$, the latter of order several hundred nanometers and much less than the channel height of 20 $\mu$m. Here $\Pi$ is the evanescent decay length of order 100 nm, as approximated using the incoming laser angle and the indices of refraction of the underlying glass, 1.52, and water in the channel, 1.33 [1]. Furthermore, $I_0$ is the intensity of a particle with center at $z = a$. Laser powers $15 \leq P_{\mathrm{laser}} \leq 150$ mW, allowed for a variation of the height, $h$, of the observation zone up to $\sim 1$ $\mu$m. The fluorescence signal emitted by the nanoparticles is collected at $\nu = 400$ Hz

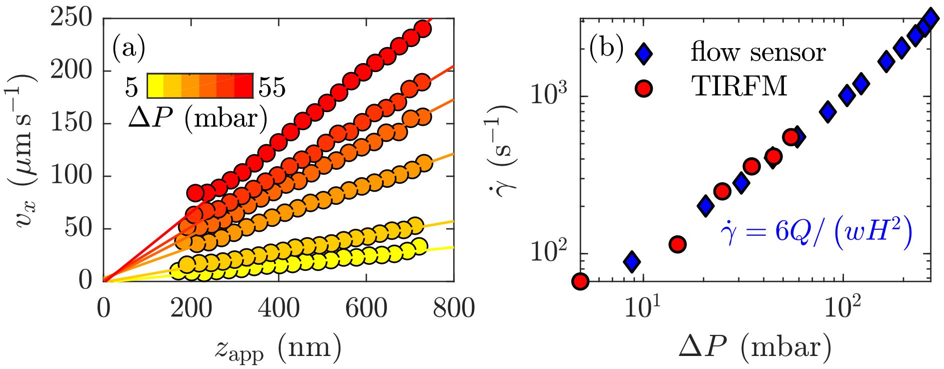


Figure S1. (a) Mean velocity profiles for nanoparticles in a NaCl aqueous solution of 5.4 mg/L and a laser power of 150 mW. The slopes give the extracted shear rates $\dot{\gamma} = \partial_z v_x$. (b) Shear-rate values measured from the velocity profiles obtained by the TIRFM technique, and with a flow sensor considering a total height of the PDMS channel $H = 20\,\mu$m and width $w = 200\,\mu$m.

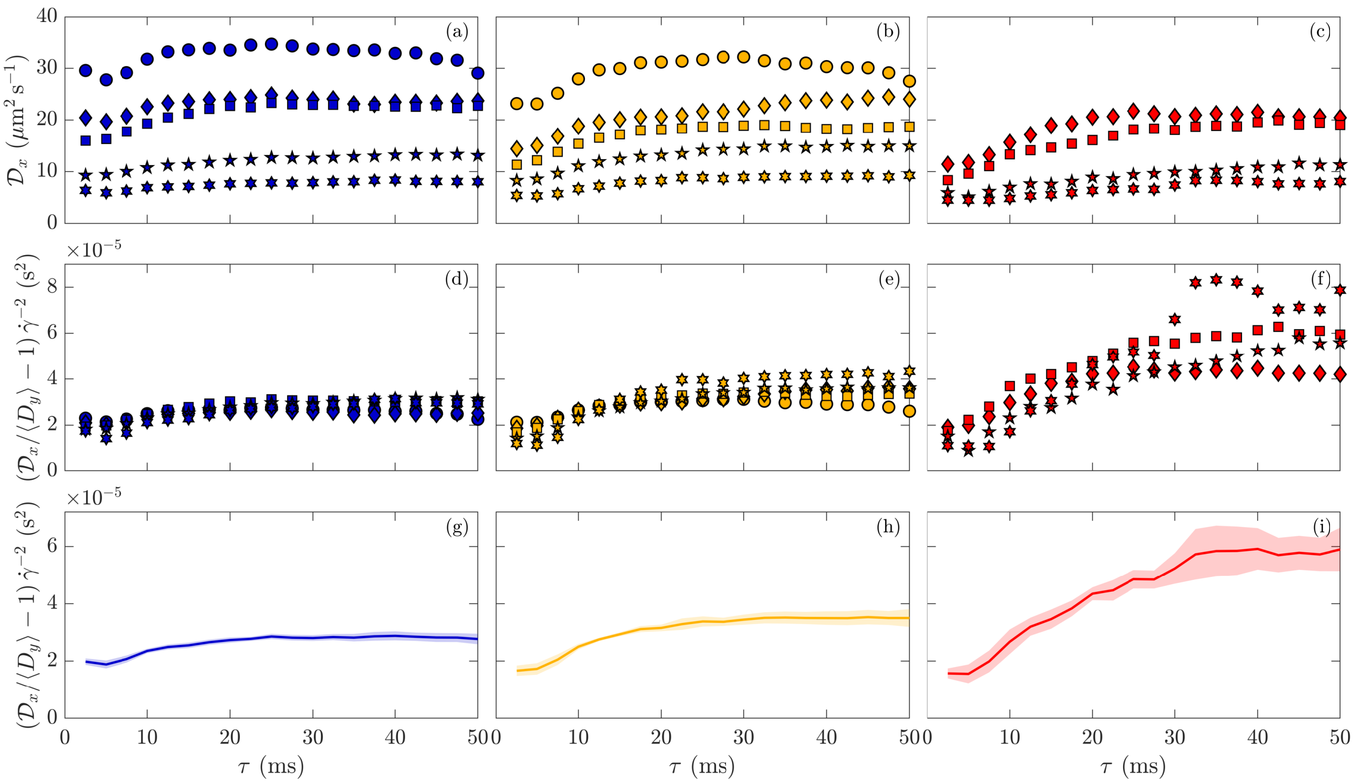


Figure S2. Dispersion coefficient measured for at least four shear rates (first row), the dimensionless, rescaled dispersion (second row), and averaged over the shear rate (third row), the latter as displayed in Fig. 2(a). The liquids used were ultrapure water (first column), $[\mathrm{NaCl} = 5.4]$ mg/L in ultra pure water (second column) and $[\mathrm{NaCl} = 54]$ mg/L (third column) in ultra pure water. The shaded areas displaye the corresponding standard deviation over the shear rates for each given delay time.

by a 16-bit camera (Andor Neo-SCMOS, 6 $\mu$m pixel size). With this camera and the objective used (Leica 100X, NA $= 1.46$), the center-of-mass positions of diffraction-limited particle images are resolved to within roughly 10 nm. Between frames, such particles are expected to diffuse an approximate distance $\sqrt{2D_0/\nu} \approx 140$ nm, which is well above the resolution of the position measurement.

## C. Particle tracking and velocity profiles

A home-made MATLAB tracking algorithm (see video S1, SI) followed $10^5$ particle trajectories; ensembles of *ca.* $10^2$ such trajectories with three delay times per column are shown in Fig. 1(b). From these ensemble trajectories, the averaged, near-wall velocity profiles $v_x(z) = \dot\gamma z$ are obtained as seen in Fig. S1. Similarly, the variance of the displacements, $\sigma_{\Delta x}$ and $\sigma_{\Delta y}$, are obtained (*cf.* Fig. 1(b)) as in our previous study [2]. Under our experimentally imposed pressures, and due to the geometry of the microchannels used, particles are advected by a laminar Poiseuille flow throughout the whole channel. Since the evanescent wave only illuminates the fluorescent particles located up to 1 $\mu$m from the lower glass surface, however, the observed near-surface flow is well-described as linear, as schematically indicated in Fig. 1(a). Indeed, Fig S1(a) shows these linear velocity profiles for several pressure drops. A linear regression allows to obtain the shear rate values $\dot\gamma$ used in the main article. These values are consistent with the ones independently inferred using a flow sensor (Elveflow MFS), as shown in Fig S1(b). To make the comparison, we assume a Poiseuille flow in the channel which can be integrated over the cross section to relate the flow rate to the near-wall shear rate, see inset equation.

## D. Scaling of the dispersion coefficients

The dispersion coefficients were measured for at least four pressure drops (*i.e.* shear rates) per set of experimental salt concentration and laser power. Since in Fig. 2(a), we only show the rescaled data, we here present the unscaled

and scaled data together. In Figure S2(a-c) are shown the raw dispersion coefficients $\mathcal{D}_x = \sigma^2_{\Delta x}/(2\tau)$ as a function of delay time $\tau$ since a particle's first observation in a trajectory. Here we show only the measurements for the largest laser power, *i.e.* 150 mW, noting similarly behavior for each of the laser powers studied.

As detailed in our previous study [2], the dispersion coefficient varies quadratically with the shear rate for the Taylor dispersion occurring in linear shear flows. Such a scaling is here again confirmed by our data in Figs S2(d-f). Consequently, the dispersion coefficients are averaged over the shear rates as displayed individually in Figs S2(g-i), and as also seen in Figure 2(a).

## III. MOMENT THEORY

### A. Advection-diffusion model

We aim at describing theoretically the transport properties and the distribution of the nanoparticles in the near-surface region of the evanescently-illuminated channels described in § II. We adopt a probabilistic description and the center-of-mass position of the nanoparticles are described in terms of probability distribution functions or concentration fields, denoted $c$. The particle volume fraction is small enough in the experiments, to neglect any hydrodynamic interactions between the particles. The channel is wide enough such that the flow is mainly in the $x$ direction and well described by a linear shear flow near the surface. For simplicity, the transport in the $y$ direction will not be considered in the present 2d ($xz$) theoretical description, as it only results from molecular diffusion [2] and we rather focus on the streamwise dispersion. The nanoparticles and the glass surfaces are negatively charged (see Fig. 1(a) in the manuscript) so that the particle are submitted to electrostatic interactions, which generate an external force $-U'_{\mathrm{el}}(z)$ on the particles, where $U_{\mathrm{el}}$ is a DLVO energy potential defined in Eq. (1) of the main text. We stress that the salt concentration used experimentally was small enough such that no adsorption of particles on the glass surface has been observed. Therefore, the van der Waals contribution in the DLVO potential is also neglected here. The concentration field follows the Fokker-Planck equation

$$\frac{\partial c}{\partial t} + v_x(z)\frac{\partial c}{\partial x} = D_x(z)\frac{\partial^2 c}{\partial x^2} + \frac{\partial}{\partial z}\left(D_z(z)\left[\frac{\partial c}{\partial z} + \frac{U'_{\mathrm{el}}(z)}{kT}c\right]\right), \tag{S1}$$

where $D_x, D_z$ are the diffusion constants. The friction drag on a particle moving near a wall increases with respect to its bulk value. As a result of these *hydrodynamic interactions*, the mobility of such particle decreases in the vicinity of the wall, which is accounted for here through the spatial dependence of the diffusion coefficients. Following Ref. [3], the diffusion coefficients of a spherical particles near a no-slip planar surface can be approximated by

$$\frac{D_x(z)}{D_0} \simeq 1 - \frac{9}{16}\frac{a}{z} + \frac{1}{8}\left(\frac{a}{z}\right)^3 - \frac{45}{256}\left(\frac{a}{z}\right)^4 - \frac{1}{16}\left(\frac{a}{z}\right)^5, \tag{S2a}$$

$$\frac{D_z(z)}{D_0} \simeq \frac{6(z-a)^2 + 2(z-a)a}{6(z-a)^2 + 9(z-a)a + 2a^2}, \tag{S2b}$$

where $z$ is the center-of-mass altitude of the particle.

The particles are tracked in the channel by using evanescent-wave microscopy. Because of the finite sensitivity of the camera, particles beyond a certain distance $h$ from the wall are not detected as their resulting fluorescence intensity is too small. The consequence is that the particles leave the field of the microscope by diffusing vertically above the altitude $z = h$. Our model assumes that the experimental trajectories are equivalent to a physical process where particles reaching the boundary of the observation zone at $z = h$ are instantaneously and permanently adsorbed, and are thus no longer considered in the ensemble. This implies a boundary condition of the probability distribution as

$$c(x, z, t) = 0, \quad \text{at} \quad z = h, \tag{S3}$$

which is equivalent to an absorption condition with an infinite absorption rate [4].

The impermeability condition at the bottom wall imposes that the mass flux vanishes there, which reads:

$$D_z(z)\left[\frac{\partial c}{\partial z} + \frac{U'_{\mathrm{el}}(z)}{kT}c\right] = 0, \quad \text{at} \quad z = a, \tag{S4}$$

where the sphere is in contact with the bottom wall. The channel is long enough to be invariant by translation along the streamwise direction. Therefore, the meaningful statistical transport quantity is the displacement with respect

to the first appearance of the particle in the channel $\Delta x = x(t+\tau) - x(t)$, which amounts to shift independent trajectories in order to start from a common spatio-temporal origin (see SM Video 2). The probability distribution is then initially located at a given horizontal position of the channel and with a certain initial distribution along $z$ as $c(x,z,t=0) = c_{\rm ini}(z)\delta(x)$, where $\delta(x)$ is the Dirac distribution.

We note that the system considered here is intrinsically out of equilibrium in the sense that the number of particles is not conserved. Therefore, the Fokker-Planck equation shown in Eq. (S1) does not have a trivial steady-state solution in contrast with Ref. [5]. Assuming that the concentration vanishes as $|x| \to \infty$ such that $\lim_{x\to\pm\infty} x^\mu \partial_x^\nu c = 0$ for arbitrary integers $\mu$, $\nu$, the moments of the distribution [6] are defined as

$$c_p(z,t) = \int_{\mathbb{R}} x^p c(x,z,t)\,\mathrm{d}x \quad \text{and} \quad m_p(t) = \int_a^h c_p(z,t)\,\mathrm{d}z \ . \tag{S5}$$

Integrating Eq. (S1), one can show that the $p^{\rm th}$ moment follows the recursive equation

$$\left(\frac{\partial}{\partial t} - \frac{\partial}{\partial z}\left(D_z(z)\left[\frac{\partial}{\partial z} + \frac{\phi'(z)}{k_{\rm B}\Theta}\right]\right)\right) c_p(z,t) = p(p-1)D_x(z)c_{p-2}(z,t) + pv_x(z)\,c_{p-1}(z,t) \ . \tag{S6}$$

From Eq. (S6), the following strategy consists in computing the time-dependent moment $c_p(z,t)$ recursively for $p = 0,1,2,....$ The transport coefficients (*i.e.* drift and dispersion coefficient) are related to the corresponding moments of the distribution as described in detail in the following.

### B. Zeroth moment and altitude probability distribution

Evaluating Eq. (S6) for $p=0$, we find that the zeroth moment $c_0$ verifies

$$\left(\frac{\partial}{\partial t} - \frac{\partial}{\partial z}\left(D_z(z)\left[\frac{\partial}{\partial z} + \frac{U'_{\rm el}(z)}{kT}\right]\right)\right) c_0(z,t) = 0 \ , \tag{S7}$$

with an initial condition $c_0(z,t=0) = c_{\rm ini}(z)$. We search for a separable solution, and inject the ansatz $c_0(z,t) = f(z)\exp(-\lambda t)$ in Eq. (S7). The solutions satisfy

$$\left[\lambda + \frac{\mathrm{d}}{\mathrm{d}z}\left(D_z(z)\left[\frac{\mathrm{d}}{\mathrm{d}z} + \frac{U'_{\rm el}(z)}{kT}\right]\right)\right] f(z) = 0 \ , \tag{S8}$$

together with the boundary conditions

$$D_z(z)\left[\frac{\mathrm{d}}{\mathrm{d}z} + \frac{U'_{\rm el}(z)}{kT}\right] f(z) = 0 \ , \qquad z = a \ , \tag{S9}$$

$$f(z) = 0 \ , \qquad z = h \ . \tag{S10}$$

By setting $p(z) = D_z(z)/c_{\rm B}(z)$, $w(z) = 1/c_{\rm B}(z)$ and $q(z) = -[D_z(z)U''_{\rm el}(z) + D'(z)U'_{\rm el}(z)]/c_{\rm B}(z)$, one can show that Eq. (S8), takes the form of a Sturm-Liouville equation [7]

$$-\Big(p(z)f'(z)\Big)' + q(z)f(z) = \lambda w(z)f(z) \ , \tag{S11}$$

where $c_{\rm B}$ is the Boltzmann distribution

$$c_{\rm B}(z) = \frac{\exp\left(-\frac{U_{\rm el}(z)}{kT}\right)}{\int_a^H \exp\left(-\frac{U_{\rm el}(z')}{kT}\right)\mathrm{d}z'} \ . \tag{S12}$$

Using results from eigenvalue theory, Eq. (S8) has a countable ensemble of solutions $(\lambda_k, f_k(z))_{k\in\mathbb{N}^*}$ that satisfies the boundary conditions Eq. (S9) and (S10), where $0 < \lambda_1 < \lambda_2 < ... < \infty$. The eigenvalues are orthogonal under the definition of the scalar product

$$\langle f,g\rangle = \int_a^H f(z)g(z)w(z)\,\mathrm{d}z = \int_a^H \frac{1}{c_{\rm B}(z)} f(z)g(z)\,\mathrm{d}z \ . \tag{S13}$$

The general solution of Eq. (S7) with its initial condition is

$$c_0(z,t) = \sum_{k\in\mathbb{N}^*} a_{0,k} f_k(z) \exp(-\lambda_k t) \ , \qquad a_{0,k} = \langle c_{\rm ini}, f_k\rangle \ , \tag{S14}$$

where $f_k$ are taken to be normalized, *i.e.* $\langle f_k, f_k\rangle = 1$. Then integrating Eq. (S14), we find that the total mass of particles, characterized by $m_0(t)$, is given by

$$m_0(t) = \sum_{k\in\mathbb{N}^*} a_{0,k} \overline{f_k} \exp(-\lambda_k t), \tag{S15}$$

and decays over time. The time-dependent altitude probability distribution (see Fig. 3(b) of the main text) are related to the zeroth-moment via

$$\mathcal{P}(z,t) = \frac{\int c(x,z,t){\rm d}x}{\int c(x,z',t){\rm d}x{\rm d}z'} = \frac{c_0(z,t)}{m_0(t)}. \tag{S16}$$

We note that the theoretical initial distribution is normalized, *i.e.* $\int_a^h c_{\rm ini}(z){\rm d}z = 1$, such that the $m_0(t)$ corresponds to the fraction of particles remaining in the observation zone, as plotted in Fig. 3(d) of the main text. The eigenvalue $\lambda_k$ and eigenfunction $f_k$ are evaluated numerically using a home-made version of the SLEIGN2 code described in Ref. [7].

### C. First moment and drift coefficient

Evaluating Eq. (S6) for $p = 1$, the governing equation for the first moment $c_1$ is

$$\left(\frac{\partial}{\partial t} - \frac{\partial}{\partial z}\left(D_z(z)\left[\frac{\partial}{\partial z} + \frac{U'_{\rm el}(z)}{kT}\right]\right)\right) c_1(z,t) = v_x(z) c_0(z,t) \ , \tag{S17}$$

with $c_1(z, t = 0) = 0$. The latter equation can be solved using again the eigenvalue theory [6] and its general solution is of the form

$$c_1(z,t) = \sum_{k\in\mathbb{N}^*} \Big(a_{1,k} f_k(z) + a_{0,k}[\zeta_k(z) + \gamma_{1,k} t f_k(z)]\Big) \exp(-\lambda_k t) \ , \tag{S18}$$

where $\zeta_k$ are the solutions of

$$-\left[\lambda_k + \frac{\rm d}{{\rm d}z}\left(D_z(z)\left[\frac{\rm d}{{\rm d}z} + \frac{U'_{\rm el}(z)}{kT}\right]\right)\right]\zeta_k(z) = \Big(v_x(z) - \gamma_{1,k}\Big) f_k(z) \ , \tag{S19}$$

with the same boundary conditions as in Eqs. (S9) and (S10). The function $\zeta_k$ can be expanded on the basis of $f_k$ as $\zeta_k = \sum_{j\in\mathbb{N}^*} A_{kj} f_j$, such that we can write the solutions as

$$c_1(z,t) = \sum_{k,j\in\mathbb{N}^{*2}} \left[\Big(a_{0,k}\gamma_{1,k} t + a_{1,k}\Big)\delta_{kj} + a_{0,k} A_{kj}\right] f_j(z) \exp(-\lambda_k t) \ , \tag{S20}$$

where $\delta_{ij}$ is the Kronecker symbol. The solvability condition imposes that the right hand side of Eq. (S19) is orthogonal to the functions $f_{j\neq k}$, which implies $\gamma_{1,k} = \langle f_k, v_x f_k\rangle$. Introducing the expansion of $\zeta_k$ in Eq. (S19), the matrix coefficients $A_{kj}$ can be evaluated as

$$A_{kj} = -\frac{(1-\delta_{jk})}{\lambda_k - \lambda_j}\langle f_j, v_x f_k\rangle \ , \tag{S21}$$

where $A_{kk}$ are arbitrary constant and have been set to zero. Finally, the initial condition sets $a_{1,k} = -\sum_{j\in\mathbb{N}^*} a_{0,j} A_{jk}$. Integrating Eq. (S18) vertically, we find the vertical-averaged first moment

$$\begin{aligned} m_1(t) &= \sum_{k\in\mathbb{N}^*} \left[a_{1,k}\overline{f_k} + a_{0,k}\gamma_{1,k} t \overline{f_k} + a_{0,k}\overline{\zeta_k}\right] \exp(-\lambda_k t) \ , \\ &= \sum_{k,j\in\mathbb{N}^{*2}} \left[\Big(a_{0,k}\gamma_{1,k} t + a_{1,k}\Big)\delta_{kj} + a_{0,k} A_{kj}\right] \overline{f_j} \exp(-\lambda_k t) \ . \end{aligned} \tag{S22}$$

The average distance $\langle x\rangle$ traveled by the particle remaining in the observation zone can be expressed as

$$\langle x\rangle = \frac{\int x c(x,z,t)\,\mathrm{d}x\mathrm{d}z}{\int c(x,z,t)\,\mathrm{d}x\mathrm{d}z} = \frac{m_1(t)}{m_0(t)}\ , \tag{S23}$$

which allows us to find a closed expression for the average drift velocity of the particles observed in the channel $\langle V\rangle = \langle x\rangle/t$.

### D. Second moment and dispersion coefficient

Considering Eq. (S6) for $p=2$, the governing partial-differential equation reads

$$\left(\frac{\partial}{\partial t} - \frac{\partial}{\partial z}\left(D_z(z)\left[\frac{\partial}{\partial z} + \frac{U'_{\mathrm{el}}(z)}{kT}\right]\right)\right) c_2(z,t) = 2D_x(z)c_0(z,t) + 2v_x(z)c_1(z,t)\ , \tag{S24}$$

with $c_2(z,t=0)=0$. The solution of the latter equation is more tedious to find than the solution of the first moment, but it relies on the same method as in the previous section. We seek for solutions of the form:

$$c_2(z,t) = \sum_{k\in\mathbb{N}^*}\left(a_{2,k}f_k(z) + \psi_k(z) + \gamma_{2,k}tf_k(z) + a_{0,k}\gamma_{1,k}t\left[2\zeta_k(z) + \gamma_{1,k}tf_k(z)\right]\right)e^{-\lambda_k t}\ , \tag{S25}$$

where $\psi_k$ are solution of

$$\begin{aligned}-\left[\lambda_k + \frac{\mathrm{d}}{\mathrm{d}z}\left(D_z(z)\left[\frac{\mathrm{d}}{\mathrm{d}z} + \frac{U'_{\mathrm{el}}(z)}{kT}\right]\right)\right]\psi_k(z) =& 2a_{0,k}D_x(z)f_k(z) - \gamma_{2,k}f_k(z)\\ &+ 2\Big(a_{1,k}v_x(z)f_k(z) + a_{0,k}(v_x(z)-\gamma_{1,k})\zeta_k(z)\Big)\ ,\end{aligned} \tag{S26}$$

with the boundary conditions Eqs. (S9) and (S10). Here again, we expand $\psi_k$ in the basis of $f_j$, *i.e.* $\psi_k(z) = \sum_{j=1}^{\infty} B_{kj}f_j(z)$, and find the corresponding coefficients using the solvability condition and initial condition as

$$\gamma_{2,k} = 2a_{0,k}\langle f_k, D_x f_k\rangle + 2a_{1,k}\langle f_k, v_x f_k\rangle + 2a_{0,k}\langle f_k, (v_x-\gamma_{1,k})\zeta_k\rangle\ , \tag{S27a}$$

$$B_{kj} = -\frac{(1-\delta_{jk})}{\lambda_k-\lambda_j}\Big[2a_{0,k}\langle f_j, D_x f_k\rangle + 2a_{1,k}\langle f_j, v_x f_k\rangle + 2a_{0,k}\langle f_j, (v_x-\gamma_{1,k})\zeta_k\rangle\Big]\ , \tag{S27b}$$

$$a_{2,k} = -\sum_{j\in\mathbb{N}^*} B_{jk}\ , \tag{S27c}$$

Integrating Eq. (S25) across the observation area, we can find the vertical-averaged second moment

$$\begin{aligned}m_2(t) &= \sum_{k\in\mathbb{N}^*}\left(a_{2,k}\overline{f_k} + \overline{\psi_k} + \gamma_{2,k}t\overline{f_k} + a_{0,k}\gamma_{1,k}t\left[2\overline{\zeta_k} + \gamma_{1,k}t\overline{f_k}\right]\right)e^{-\lambda_k t}\\ &= \sum_{k,j\in\mathbb{N}^{*2}}\left[\left(a_{2,k} + \gamma_{2,k}t + a_{0,k}\gamma_{1,k}^2t^2\right)\delta_{kj} + 2a_{0,k}\gamma_{1,k}A_{k,j}t + B_{k,j}\right]\overline{f_j}e^{-\lambda_k t}.\end{aligned} \tag{S28}$$

The variance of the distribution in the streamwise direction is defined as

$$\langle(x-\langle x\rangle)^2\rangle = \frac{\int x^2 c(x,z,t)\,\mathrm{d}x\mathrm{d}z}{\int c(x,z,t)\,\mathrm{d}x\mathrm{d}z} - \left(\frac{\int x c(x,z,t)\,\mathrm{d}x\mathrm{d}z}{\int c(x,z,t)\,\mathrm{d}x\mathrm{d}z}\right)^2, \tag{S29}$$

such that the dispersion coefficient reads

$$\mathcal{D}_x = \frac{\langle(x-\langle x\rangle)^2\rangle}{2t} = \frac{1}{2t}\left(\frac{m_2(t)}{m_0(t)} - \frac{m_1^2(t)}{m_0^2(t)}\right). \tag{S30}$$

### E. Long-time asymptotic expression

As shown above, the moments of the concentration field are found to follow a modal decomposition $c_p(z,t) = \sum_{k=1}^{\infty} c_{p,k}(z,t)\exp(-\lambda_k t)$, where $c_{p,k}$ are polynomial functions of $t$ of degree $p$, and where $0 < \lambda_1 < \lambda_2 < \cdots$. Therefore, there is no steady-state solution and the concentration fields decays to zero at long times. Nevertheless, in the long-time limit, the concentration is governed by the slowest relaxation mode $\lambda_1$, and the probability density function of particles remaining in the channel converges toward a steady state. For time larger than $t \gg \frac{1}{\lambda_2-\lambda_1}$, we truncate the expansion to its leading order and the moments $c_{p\leq 2}$ follow

$$c_0(z,t) \simeq a_{0,1} f_1(z) e^{-\lambda_1 t} , \tag{S31}$$

$$c_1(z,t) \simeq \left(a_{1,1} f_1(z) + a_{0,1}[\zeta_1(z) + t\gamma_{1,1} f_1(z)]\right) e^{-\lambda_1 t} , \tag{S32}$$

$$c_2(z,t) \simeq \left(a_{2,1} f_1(z) + \psi_1(z) + t\gamma_{2,1} f_1(z) + t a_{0,1}\gamma_{1,1}\left[2\zeta_1(z) + t\gamma_{1,1} f_1(z)\right]\right) e^{-\lambda_1 t} . \tag{S33}$$

Similarly, the vertical-averaged moments can be truncated to

$$m_0(t) \simeq a_{0,1}\overline{f_1} e^{-\lambda_1 t} , \tag{S34}$$

$$m_1(t) \simeq \left(a_{1,1}\overline{f_1} + a_{0,1}[\overline{\zeta_1} + t\gamma_{1,1}\overline{f_1}]\right) e^{-\lambda_1 t} , \tag{S35}$$

$$m_2(t) \simeq \left(a_{2,1}\overline{f_1} + \overline{\psi_1} + t\gamma_{2,1}\overline{f_1} + t a_{0,1}\gamma_{1,1}\left[2\overline{\zeta_1} + t\gamma_{1,1}\overline{f_1}\right]\right) e^{-\lambda_1 t} . \tag{S36}$$

Introducing the latter expansion into Eq. (S16), the long-time altitude probability distribution converges toward a steady state, independent of the initial distribution and is given by

$$\mathcal{P}(z) = \frac{f_1(z)}{\overline{f_1}} , \tag{S37}$$

as observed in Fig. 3(b) of the main text. The average velocity of the particles observed in the channel also converges toward a finite value given by

$$\langle V \rangle = \frac{\langle x \rangle}{t} = \langle f_1, v_x f_1 \rangle = \int_a^h \frac{1}{c_{\mathrm{B}}(z)} f_1^2(z) v_x(z)\,\mathrm{d}z . \tag{S38}$$

The averaging here corresponds to a time average of the velocity as $\langle V \rangle = \frac{1}{t}\int_0^t v_x(z_t)\,\mathrm{d}t$, where $z_t$ denotes the vertical position at time $t$. Interestingly, the long-time asymptotic time-average velocity of particle $\langle x \rangle/t$ differs from the ensemble-average velocity $\langle v_x \rangle$ of particles remaining in the channel, which reads

$$\langle v_x \rangle = \int_a^h \mathcal{P}(z) v_x(z)\,\mathrm{d}z = \int_a^h \frac{f_1(z)}{\overline{f_1}} v_x(z)\,\mathrm{d}z . \tag{S39}$$

One would expect the two averaged velocities defined in Eqs. (S38) and (S39) to be the same from the ergodic theorem. Such a principle holds in equilibrium physics and the difference in the long-time velocity arises from the nonequilibrium nature of the problem. Finally the long-time dispersion coefficient can be computed from Eq. (S30) as

$$\mathcal{D}_x = \langle f_1, D_x f_1 \rangle + \langle f_1, (v_x - \langle V \rangle)\zeta_1 \rangle = \int_a^h \frac{1}{c_{\mathrm{B}}(z)} f_1^2(z) D_x(z)\,\mathrm{d}z + \int_a^h \frac{1}{c_{\mathrm{B}}(z)} (v_x(z) - \langle V \rangle)\zeta_1(z) f_1(z)\,\mathrm{d}z . \tag{S40}$$

which corresponds to the Eq. (4) of the manuscript and is the main theoretical result of this work. In a similar fashion as in Taylor-Aris theory, the dispersion takes the form of the sum of the molecular diffusion contribution and the advection-diffusion coupling.

The latter expression accounts for various nanoscale effects such as electrostatic interactions, hydrodynamic interactions and the absorbing condition. To illustrate the importance of these different mechanisms, we focus on two limiting cases of no interactions in Section III F and reflective boundary conditions in Section III G. Finally, the Section III H summarizes the different cases in correspondance to the Fig. 4(b) of the manuscript.

### F. Tracer non-interacting particles

An interesting case is the limit of point-like tracer particles when interactions can be neglected. We suppose that the radius of the particle is small with respect to the channel size, *i.e.* $a/h \to 0$. The typical length scale of variation of the diffusion constants due to the hydrodynamic interactions is given by the radius of the particle such that we neglect the spatial variation of $D_x$ and $D_z$. Furthermore, we ignore here the effect external forces, meaning that $U_{\rm el}(z) = 0$. In that case, the Eq. (S8) simplifies and can be computed exactly with its boundary condition Eqs. (S9) and (S10). The first mode is described by

$$\lambda_1 = \frac{\pi^2 D_0}{4h^2} \ , \qquad f_1(z) = \frac{\sqrt{2}}{h}\cos\left(\frac{\pi z}{2h}\right) \ , \qquad c_{\rm B}(z) = \frac{1}{h} \ . \tag{S41}$$

Using this expression in Eq. (S40), we compute exactly the steady-state average drift velocity and dispersion coefficient

$$\langle V\rangle = \left(1 - \frac{2}{\pi^2}\right)\frac{\dot\gamma h}{2} \approx 0.29736\,\dot\gamma h, \qquad \mathcal{D}_x = D_0 + \frac{240 - 12\pi^2 - \pi^4}{3\pi^6}\frac{\dot\gamma^2 h^4}{4D_0} \approx D_0\left(1 + 0.0083753\ {\rm Pe}^2\right) \ . \tag{S42}$$

This latter result can be compared, as in Fig. 4(b) of the main text, to the classical, Taylor-Aris tracer result for reflecting boundaries on both the top and bottom of the channel. Recalling the discussion preceding Eq. (1) of the main text, the Taylor-Aris result is $\mathcal{D}_x^{\rm TA} = D_0\left(1 + 30^{-1}\ {\rm Pe}^2\right)$, or, a factor of approximately four separating reflecting and absorbing walls for linear shear flows.

### G. Dispersion coefficient in a 2d channel with reflecting boundary condition

The long-time dispersion coefficient in the case of a channel of size $h$ with reflecting boundary conditions at both interfaces can be found using the formalism derived here. In this situation, the altitude probability distribution has a stationary solution, which is given the Gibbs-Boltzmann distribution as $c_0(z, t \to \infty) = c_{\rm B}(z)$, and that corresponds to the trivial solution of the eigenvalue problem Eq. (S8) as $\lambda_1 = 0$, $f_1(z) = c_{\rm B}(z)$, which is not the general case for absorption. Injecting the latter in Eq. (S19), the stationary eigenmode $\zeta_1$ can be expressed as

$$\zeta_1(z) = -c_{\rm B}(z)\int_a^z \frac{{\rm d}z'}{c_{\rm B}(z')D_z(z')}\int_a^{z'} \left[v_x(z'') - \langle V\rangle\right] c_{\rm B}(z''){\rm d}z'', \tag{S43}$$

where the long-time averaged drift velocity is here $\langle V\rangle = \int_a^h c_{\rm B}(z) v_x(z)\,{\rm d}z$. Finally, introducing this expression in Eq. (S40) and performing an integration by part, we recover the expressions derived in Refs. [5, 8]

$$\mathcal{D}_x = \langle D_x\rangle + \int_a^h \frac{1}{D_z(z)c_{\rm B}(z)}\left[\int_a^z \left[v_x(z') - \langle V\rangle\right] c_{\rm B}(z')\,{\rm d}z'\right]^2 \ {\rm d}z \ , \tag{S44}$$

where the long-time averaged molecular diffusion is $\langle D_x\rangle = \int_a^h c_{\rm B}(z) D_x(z)\,{\rm d}z$.

### H. Model schematics

In Figure S3 we recall the models used to predict dispersion in a simple shear flow. As shown in Fig. 2(a), this dispersion depends on experimental variations of the salt concentration (particle-wall interaction) and the laser power (variation of the effective channel height) in the evanescent-wave microscopy observations reported here. Shown in the first column of Figure S3 are schematics, line styles from Fig. 4(b) and equations describing

- (a) the classical Taylor prediction [9, 10], with tracer particles and reflection conditions at the boundaries;
- (b) a model with no particle consumption, but with one interacting wall (potential and hydrodynamic interactions), derived from Refs. [5, 8] and seen in Eq. S44;
- (c) a model considering tracer particles with a consumption condition at one wall, Eq. S42;
- and (d) the full model as Eq. 4 in the main text and derived above, also in Eq. S40.

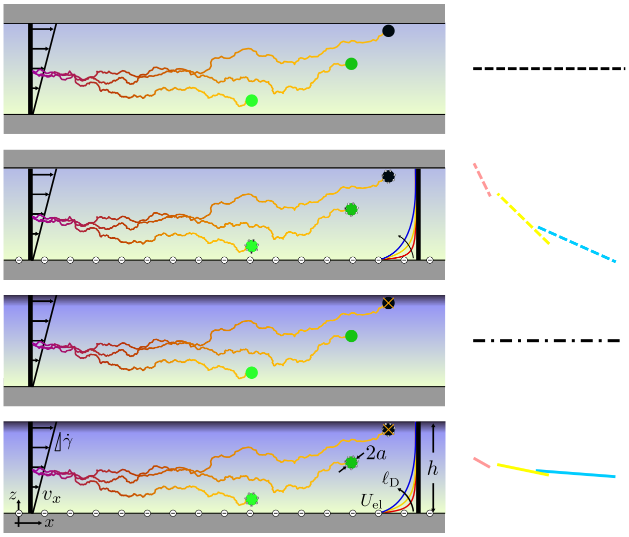


(a) $$\mathcal{D}_x = D_0 \left(1 + \frac{1}{30}\,\mathrm{Pe}^2\right)$$

(b) $$\mathcal{D}_x = \langle D_x \rangle + \int_a^h \frac{1}{D_z(z) c_\mathrm{B}(z)} \left[\int_a^z \left[v_x\left(z'\right) - \langle V \rangle\right] c_\mathrm{B}\left(z'\right) \mathrm{d}z'\right]^2 \mathrm{d}z$$

(c) $$\mathcal{D}_x \approx D_0 \left(1 + 0.0083753\ \mathrm{Pe}^2\right)$$

(d) $$\mathcal{D}_x = \langle D_x \rangle + \int_a^h \frac{1}{c_\mathrm{B}(z)} \left[v_x(z) - \langle V \rangle\right] \zeta_1(z) f_1(z)\ \mathrm{d}z$$

Figure S3. Schematics (left column); line style of Fig. 4 of the main text (central column); and dispersion predicition (right column) for the different models described in the text.

[1] Lukas Novotny and Bert Hecht, *Principles of nano-optics* (Cambridge University Press, Cambridge ; New York, 2006).
[2] Alexandre Vilquin, Vincent Bertin, Pierre Soulard, Gabriel Guyard, Elie Raphaël, Frédéric Restagno, Thomas Salez, and Joshua D. McGraw, "Time dependence of advection-diffusion coupling for nanoparticle ensembles," Phys. Rev. Fluids **6**, 064201 (2021).
[3] Zhenzhen Li, Loïc D'eramo, Choongyeop Lee, Fabrice Monti, Marc Yonger, Patrick Tabeling, Benjamin Chollet, Bruno Bresson, and Yvette Tran, "Near-wall nanovelocimetry based on total internal reflection fluorescence with continuous tracking," Journal of Fluid Mechanics **766**, 147–171 (2015).
[4] Rudro R Biswas and Pabitra N Sen, "Taylor dispersion with absorbing boundaries: A stochastic approach," Physical review letters **98**, 164501 (2007).
[5] Howard Brenner and Lawrence J Gaydos, "The constrained brownian movement of spherical particles in cylindrical pores of comparable radius: models of the diffusive and convective transport of solute molecules in membranes and porous media," Journal of Colloid and Interface Science **58**, 312–356 (1977).
[6] NG Barton, "An asymptotic theory for dispersion of reactive contaminants in parallel flow," The ANZIAM Journal **25**, 287–310 (1984).
[7] Paul B Bailey, William N Everitt, and Anton Zettl, "The sleign2 sturm-liouville code," ACM Trans. Math. Software **27**, 143–192 (2001).
[8] Arthur Alexandre, Thomas Guérin, and David S Dean, "Generalized taylor dispersion for translationally invariant microfluidic systems," Physics of Fluids **33**, 082004 (2021).
[9] Geoffrey Ingram Taylor, "Dispersion of soluble matter in solvent flowing slowly through a tube," Proceedings of the Royal Society of London. Series A. Mathematical and Physical Sciences **219**, 186–203 (1953).
[10] Rutherford Aris, "On the dispersion of a solute in a fluid flowing through a tube," Proceedings of the Royal Society of London. Series A. Mathematical and Physical Sciences **235**, 67–77 (1956).
